# Supplementary material for: Double-Differential Inclusive Charged-Current $\nu_\mu$ Cross Sections on Hydrocarbon in MINERvA at $\langle E_{\nu} \rangle \sim$ 3.5 GeV
Source: arXiv:2002.12496 ancillary file (2020-06-23)
Supplement: Supplementary file 1 [file SupplementaryMaterial.pdf]

# Double-Differential Inclusive Charged-Current $\nu_\mu$ Cross Sections on Hydrocarbon in MINERvA at $\langle E_\nu \rangle \sim 3.5$ GeV

A. Filkins,<sup>1</sup> D. Ruterbories,<sup>2</sup> Y. Liu,<sup>1</sup> Z. Ahmad Dar,<sup>3</sup> F. Akbar,<sup>3</sup> O. Altinok,<sup>4</sup> D.A. Andrade,<sup>5</sup> M. V. Ascencio,<sup>6</sup> A. Bashyal,<sup>7</sup> A. Bercellie,<sup>2</sup> M. Betancourt,<sup>8</sup> A. Bodek,<sup>2</sup> J. L. Bonilla,<sup>5</sup> A. Bravar,<sup>9</sup> H. Budd,<sup>2</sup> G. Caceres,<sup>10</sup> T. Cai,<sup>2</sup> M.F. Carneiro,<sup>7,10,\*</sup> H. da Motta,<sup>10</sup> S.A. Dytman,<sup>11</sup> G.A. Díaz,<sup>2,6</sup> J. Felix,<sup>5</sup> L. Fields,<sup>8</sup> R. Fine,<sup>2</sup> A.M. Gago,<sup>6</sup> H. Gallagher,<sup>4</sup> A. Ghosh,<sup>12,10</sup> R. Gran,<sup>13</sup> D.A. Harris,<sup>14,8</sup> S. Henry,<sup>2</sup> S. Jena,<sup>15</sup> D. Jena,<sup>8</sup> J. Kleykamp,<sup>2</sup> M. Kordosky,<sup>1</sup> D. Last,<sup>16</sup> T. Le,<sup>4,17</sup> J. LeClerc,<sup>18</sup> A. Lozano,<sup>10</sup> X.-G. Lu,<sup>19</sup> E. Maher,<sup>20</sup> S. Manly,<sup>2</sup> W.A. Mann,<sup>4</sup> C. Mauger,<sup>16</sup> K.S. McFarland,<sup>2</sup> A.M. McGowan,<sup>2</sup> B. Messerly,<sup>11</sup> J. Miller,<sup>12</sup> J.G. Morfin,<sup>8</sup> J.K. Nelson,<sup>1</sup> C. Nguyen,<sup>18</sup> A. Norrick,<sup>1</sup> A. Olivier,<sup>2</sup> V. Paolone,<sup>11</sup> G.N. Perdue,<sup>8,2</sup> M.A. Ramírez,<sup>5</sup> R.D. Ransome,<sup>17</sup> H. Ray,<sup>18</sup> H. Schellman,<sup>7</sup> C.J. Solano Salinas,<sup>21</sup> H. Su,<sup>11</sup> M. Sultana,<sup>2</sup> V.S. Syrotenko,<sup>4</sup> E. Valencia,<sup>1,5</sup> M. Wospakrik,<sup>18</sup> C. Wret,<sup>2</sup> B. Yaeggy,<sup>12</sup> and L. Zazueta<sup>1</sup>

(The MINERvA Collaboration)

<sup>1</sup>*Department of Physics, College of William & Mary, Williamsburg, Virginia 23187, USA*

<sup>2</sup>*University of Rochester, Rochester, New York 14627 USA*

<sup>3</sup>*AMU Campus, Aligarh, Uttar Pradesh 202001, India*

<sup>4</sup>*Physics Department, Tufts University, Medford, Massachusetts 02155, USA*

<sup>5</sup>*Campus León y Campus Guanajuato, Universidad de Guanajuato, Lascruain de Retana No. 5, Colonia Centro, Guanajuato 36000, Guanajuato México.*

<sup>6</sup>*Sección Física, Departamento de Ciencias, Pontificia Universidad Católica del Perú, Apartado 1761, Lima, Perú*

<sup>7</sup>*Department of Physics, Oregon State University, Corvallis, Oregon 97331, USA*

<sup>8</sup>*Fermi National Accelerator Laboratory, Batavia, Illinois 60510, USA*

<sup>9</sup>*University of Geneva, 1211 Geneva 4, Switzerland*

<sup>10</sup>*Centro Brasileiro de Pesquisas Físicas, Rua Dr. Xavier Sigaud 150, Urca, Rio de Janeiro, Rio de Janeiro, 22290-180, Brazil*

<sup>11</sup>*Department of Physics and Astronomy, University of Pittsburgh, Pittsburgh, Pennsylvania 15260, USA*

<sup>12</sup>*Departamento de Física, Universidad Técnica Federico Santa María, Avenida España 1680 Casilla 110-V, Valparaíso, Chile*

<sup>13</sup>*Department of Physics, University of Minnesota – Duluth, Duluth, Minnesota 55812, USA*

<sup>14</sup>*York University, Department of Physics and Astronomy, Toronto, Ontario, M3J 1P3 Canada*

<sup>15</sup>*Department of Physical Sciences, IISER Mohali, Knowledge City, SAS Nagar, Mohali - 140306, Punjab, India*

<sup>16</sup>*Department of Physics and Astronomy, University of Pennsylvania, Philadelphia, PA 19104*

<sup>17</sup>*Rutgers, The State University of New Jersey, Piscataway, New Jersey 08854, USA*

<sup>18</sup>*University of Florida, Department of Physics, Gainesville, FL 32611*

<sup>19</sup>*Oxford University, Department of Physics, Oxford, OX1 3PJ United Kingdom*

<sup>20</sup>*Massachusetts College of Liberal Arts, 375 Church Street, North Adams, MA 01247*

<sup>21</sup>*Universidad Nacional de Ingeniería, Apartado 31139, Lima, Perú*

(Dated: May 27, 2020)

## I. SUPPLEMENTAL MATERIALS

This supplement includes the double and single differential cross sections used in this analysis. The bin limits used for all cross sections are presented in Table I. Double differential cross sections are given in section IA, and single differential cross sections are shown in IB.

| Bin | $p_{  }$     | $p_T$          |
|-----|--------------|----------------|
| 1   | [1.5, 2.0)   | [0.000, 0.075) |
| 2   | [2.0, 2.5)   | [0.075, 0.150) |
| 3   | [2.5, 3.0)   | [0.150, 0.250) |
| 4   | [3.0, 3.5)   | [0.250, 0.325) |
| 5   | [3.5, 4.0)   | [0.325, 0.400) |
| 6   | [4.0, 4.5)   | [0.400, 0.475) |
| 7   | [4.5, 5.0)   | [0.475, 0.550) |
| 8   | [5.0, 6.0)   | [0.550, 0.700) |
| 9   | [6.0, 8.0)   | [0.700, 0.850) |
| 10  | [8.0, 10.0)  | [0.850, 1.000) |
| 11  | [10.0, 15.0) | [1.000, 1.250) |
| 12  | [15.0, 20.0) | [1.250, 1.500) |
| 13  |              | [1.500, 2.500) |

TABLE I. The binning in  $p_{||}$  and  $p_T$  used for all results.

\* Now at Brookhaven National Laboratory

### A. Double Differential Cross Sections

The measured double differential cross section is shown in Table II, with the total uncertainties Table III. Tables IV-XIII show the Monte Carlo cross sections for each model and variant used.

|    | 1        | 2        | 3        | 4        | 5        | 6        | 7        | 8        | 9        | 10       | 11       | 12       |
|----|----------|----------|----------|----------|----------|----------|----------|----------|----------|----------|----------|----------|
| 1  | 2.31e-40 | 2.34e-40 | 2.68e-40 | 1.86e-40 | 1.54e-40 | 5.68e-41 | 5.18e-41 | 3.11e-41 | 2.75e-41 | 2.86e-41 | 1.00e-41 | 5.97e-42 |
| 2  | 9.01e-40 | 1.09e-39 | 1.03e-39 | 8.10e-40 | 6.16e-40 | 3.26e-40 | 1.96e-40 | 1.52e-40 | 1.07e-40 | 5.80e-41 | 3.32e-41 | 1.39e-41 |
| 3  | 2.70e-39 | 2.57e-39 | 2.49e-39 | 2.01e-39 | 1.10e-39 | 7.55e-40 | 4.44e-40 | 3.72e-40 | 2.04e-40 | 1.35e-40 | 7.04e-41 | 2.83e-41 |
| 4  | 4.49e-39 | 4.31e-39 | 3.93e-39 | 3.33e-39 | 2.19e-39 | 1.16e-39 | 7.75e-40 | 4.96e-40 | 3.58e-40 | 2.26e-40 | 1.17e-40 | 4.56e-41 |
| 5  | 6.42e-39 | 6.18e-39 | 5.77e-39 | 4.08e-39 | 2.69e-39 | 1.55e-39 | 1.13e-39 | 7.38e-40 | 4.73e-40 | 2.91e-40 | 1.66e-40 | 6.62e-41 |
| 6  | 7.81e-39 | 7.32e-39 | 6.27e-39 | 4.94e-39 | 2.92e-39 | 1.77e-39 | 1.20e-39 | 9.09e-40 | 5.54e-40 | 3.86e-40 | 2.14e-40 | 9.06e-41 |
| 7  | 8.59e-39 | 8.12e-39 | 6.90e-39 | 5.38e-39 | 3.20e-39 | 1.88e-39 | 1.36e-39 | 9.89e-40 | 6.35e-40 | 4.06e-40 | 2.33e-40 | 9.86e-41 |
| 8  | 5.37e-39 | 8.64e-39 | 6.96e-39 | 4.96e-39 | 3.08e-39 | 2.06e-39 | 1.50e-39 | 1.11e-39 | 7.33e-40 | 4.42e-40 | 2.50e-40 | 1.06e-40 |
| 9  | 1.47e-40 | 5.22e-39 | 5.41e-39 | 3.94e-39 | 2.59e-39 | 1.84e-39 | 1.44e-39 | 1.13e-39 | 7.59e-40 | 4.81e-40 | 2.63e-40 | 1.20e-40 |
| 10 | 0.00e+00 | 3.61e-40 | 3.51e-39 | 2.95e-39 | 2.21e-39 | 1.66e-39 | 1.22e-39 | 1.11e-39 | 6.95e-40 | 4.82e-40 | 2.53e-40 | 1.20e-40 |
| 11 | 0.00e+00 | 0.00e+00 | 2.81e-40 | 1.43e-39 | 1.39e-39 | 1.20e-39 | 1.09e-39 | 8.81e-40 | 6.64e-40 | 4.29e-40 | 2.48e-40 | 1.10e-40 |
| 12 | 0.00e+00 | 0.00e+00 | 0.00e+00 | 0.00e+00 | 4.31e-40 | 7.17e-40 | 6.88e-40 | 6.45e-40 | 4.49e-40 | 3.70e-40 | 2.12e-40 | 9.30e-41 |
| 13 | 0.00e+00 | 0.00e+00 | 0.00e+00 | 0.00e+00 | 0.00e+00 | 2.29e-41 | 9.54e-41 | 1.34e-40 | 1.38e-40 | 1.32e-40 | 9.22e-41 | 5.37e-41 |

TABLE II. Measured double differential cross section as a function of  $p_{||}$  (columns) and  $p_T$  (rows) in units of  $\text{cm}^2$  per  $\text{GeV}^2$  per nucleon.

|    | 1        | 2        | 3        | 4        | 5        | 6        | 7        | 8        | 9        | 10       | 11       | 12       |
|----|----------|----------|----------|----------|----------|----------|----------|----------|----------|----------|----------|----------|
| 1  | 4.40e-41 | 3.69e-41 | 3.99e-41 | 3.06e-41 | 2.67e-41 | 1.34e-41 | 1.27e-41 | 7.71e-42 | 6.33e-42 | 6.03e-42 | 2.60e-42 | 1.67e-42 |
| 2  | 1.33e-40 | 1.23e-40 | 1.14e-40 | 9.01e-41 | 7.08e-41 | 4.36e-41 | 2.90e-41 | 2.13e-41 | 1.35e-41 | 8.98e-42 | 4.71e-42 | 2.01e-42 |
| 3  | 3.67e-40 | 2.50e-40 | 2.34e-40 | 1.68e-40 | 9.86e-41 | 7.01e-41 | 4.50e-41 | 3.55e-41 | 1.99e-41 | 1.54e-41 | 6.81e-42 | 3.18e-42 |
| 4  | 5.52e-40 | 4.51e-40 | 3.48e-40 | 2.88e-40 | 1.90e-40 | 1.07e-40 | 7.60e-41 | 4.73e-41 | 3.32e-41 | 2.28e-41 | 1.20e-41 | 4.70e-42 |
| 5  | 8.64e-40 | 5.44e-40 | 5.14e-40 | 3.23e-40 | 2.25e-40 | 1.37e-40 | 1.00e-40 | 6.60e-41 | 4.14e-41 | 2.76e-41 | 1.63e-41 | 6.13e-42 |
| 6  | 8.03e-40 | 6.64e-40 | 5.29e-40 | 3.85e-40 | 2.46e-40 | 1.59e-40 | 1.08e-40 | 7.75e-41 | 4.46e-41 | 3.53e-41 | 1.82e-41 | 7.85e-42 |
| 7  | 1.01e-39 | 7.37e-40 | 5.50e-40 | 4.24e-40 | 2.95e-40 | 1.56e-40 | 1.17e-40 | 8.24e-41 | 5.06e-41 | 3.54e-41 | 1.90e-41 | 8.49e-42 |
| 8  | 4.70e-40 | 6.87e-40 | 5.26e-40 | 3.92e-40 | 2.58e-40 | 1.71e-40 | 1.20e-40 | 8.55e-41 | 5.54e-41 | 3.51e-41 | 2.03e-41 | 8.90e-42 |
| 9  | 2.22e-41 | 4.23e-40 | 4.18e-40 | 3.42e-40 | 2.13e-40 | 1.49e-40 | 1.18e-40 | 8.80e-41 | 5.70e-41 | 3.79e-41 | 2.05e-41 | 9.94e-42 |
| 10 | 0.00e+00 | 5.22e-41 | 3.03e-40 | 2.59e-40 | 1.93e-40 | 1.43e-40 | 1.02e-40 | 8.74e-41 | 5.28e-41 | 3.82e-41 | 1.92e-41 | 1.03e-41 |
| 11 | 0.00e+00 | 0.00e+00 | 3.92e-41 | 1.50e-40 | 1.27e-40 | 1.01e-40 | 9.07e-41 | 6.98e-41 | 5.10e-41 | 3.40e-41 | 1.89e-41 | 9.65e-42 |
| 12 | 0.00e+00 | 0.00e+00 | 0.00e+00 | 0.00e+00 | 5.80e-41 | 8.66e-41 | 6.54e-41 | 5.60e-41 | 3.98e-41 | 3.12e-41 | 1.65e-41 | 8.74e-42 |
| 13 | 0.00e+00 | 0.00e+00 | 0.00e+00 | 0.00e+00 | 0.00e+00 | 3.64e-42 | 1.14e-41 | 1.73e-41 | 1.38e-41 | 1.27e-41 | 8.05e-42 | 4.79e-42 |

TABLE III. The total uncertainty on the measured double differential cross section as a function of  $p_{||}$  (columns) and  $p_T$  (rows) in units of  $\text{cm}^2$  per  $\text{GeV}^2$  per nucleon.

|    | 1        | 2        | 3        | 4        | 5        | 6        | 7        | 8        | 9        | 10       | 11       | 12       |
|----|----------|----------|----------|----------|----------|----------|----------|----------|----------|----------|----------|----------|
| 1  | 3.16e-40 | 3.54e-40 | 3.57e-40 | 2.90e-40 | 1.96e-40 | 1.11e-40 | 6.70e-41 | 4.12e-41 | 2.53e-41 | 1.80e-41 | 1.12e-41 | 5.08e-42 |
| 2  | 1.09e-39 | 1.22e-39 | 1.21e-39 | 9.87e-40 | 6.47e-40 | 3.79e-40 | 2.20e-40 | 1.38e-40 | 8.85e-41 | 5.58e-41 | 3.02e-41 | 1.29e-41 |
| 3  | 2.49e-39 | 2.58e-39 | 2.50e-39 | 2.00e-39 | 1.31e-39 | 7.63e-40 | 4.51e-40 | 2.95e-40 | 1.82e-40 | 1.14e-40 | 6.24e-41 | 2.60e-41 |
| 4  | 4.31e-39 | 4.32e-39 | 4.06e-39 | 3.20e-39 | 2.08e-39 | 1.20e-39 | 7.41e-40 | 4.71e-40 | 2.92e-40 | 1.85e-40 | 1.02e-40 | 4.22e-41 |
| 5  | 6.04e-39 | 5.94e-39 | 5.34e-39 | 4.14e-39 | 2.68e-39 | 1.56e-39 | 9.97e-40 | 6.41e-40 | 4.02e-40 | 2.53e-40 | 1.38e-40 | 5.61e-41 |
| 6  | 7.60e-39 | 7.06e-39 | 6.28e-39 | 4.72e-39 | 3.06e-39 | 1.82e-39 | 1.16e-39 | 7.74e-40 | 4.84e-40 | 3.11e-40 | 1.66e-40 | 6.98e-41 |
| 7  | 8.56e-39 | 7.72e-39 | 6.59e-39 | 4.93e-39 | 3.14e-39 | 1.91e-39 | 1.27e-39 | 8.70e-40 | 5.57e-40 | 3.53e-40 | 1.85e-40 | 7.78e-41 |
| 8  | 4.85e-39 | 7.64e-39 | 6.31e-39 | 4.57e-39 | 2.92e-39 | 1.85e-39 | 1.30e-39 | 9.34e-40 | 6.08e-40 | 3.93e-40 | 2.08e-40 | 8.62e-41 |
| 9  | 1.16e-40 | 4.70e-39 | 5.13e-39 | 3.64e-39 | 2.42e-39 | 1.65e-39 | 1.26e-39 | 9.57e-40 | 6.46e-40 | 4.20e-40 | 2.22e-40 | 9.21e-41 |
| 10 | 0.00e+00 | 3.13e-40 | 3.02e-39 | 2.54e-39 | 1.82e-39 | 1.38e-39 | 1.11e-39 | 8.93e-40 | 6.25e-40 | 4.08e-40 | 2.21e-40 | 9.44e-41 |
| 11 | 0.00e+00 | 0.00e+00 | 2.12e-40 | 1.12e-39 | 1.18e-39 | 9.98e-40 | 8.73e-40 | 7.50e-40 | 5.47e-40 | 3.73e-40 | 2.04e-40 | 9.04e-41 |
| 12 | 0.00e+00 | 0.00e+00 | 0.00e+00 | 0.00e+00 | 3.34e-40 | 5.95e-40 | 5.70e-40 | 5.19e-40 | 4.09e-40 | 2.95e-40 | 1.72e-40 | 8.15e-41 |
| 13 | 0.00e+00 | 0.00e+00 | 0.00e+00 | 0.00e+00 | 0.00e+00 | 1.88e-41 | 7.27e-41 | 1.14e-40 | 1.34e-40 | 1.21e-40 | 8.60e-41 | 5.08e-41 |

TABLE IV. Monte Carlo predicted double differential cross section as a function of  $p_{||}$  (columns) and  $p_T$  (rows) in units of  $\text{cm}^2$  per  $\text{GeV}^2$  per nucleon. This prediction is for MnvGENIE v1.

|    | 1        | 2        | 3        | 4        | 5        | 6        | 7        | 8        | 9        | 10       | 11       | 12       |
|----|----------|----------|----------|----------|----------|----------|----------|----------|----------|----------|----------|----------|
| 1  | 2.89e-40 | 3.23e-40 | 3.25e-40 | 2.63e-40 | 1.82e-40 | 1.06e-40 | 6.41e-41 | 3.78e-41 | 2.29e-41 | 1.65e-41 | 1.03e-41 | 4.80e-42 |
| 2  | 1.03e-39 | 1.16e-39 | 1.15e-39 | 9.45e-40 | 6.29e-40 | 3.68e-40 | 2.14e-40 | 1.33e-40 | 8.38e-41 | 5.33e-41 | 2.88e-41 | 1.25e-41 |
| 3  | 2.43e-39 | 2.50e-39 | 2.43e-39 | 1.97e-39 | 1.32e-39 | 7.73e-40 | 4.56e-40 | 2.91e-40 | 1.76e-40 | 1.12e-40 | 6.17e-41 | 2.56e-41 |
| 4  | 4.18e-39 | 4.15e-39 | 3.89e-39 | 3.07e-39 | 2.04e-39 | 1.20e-39 | 7.25e-40 | 4.56e-40 | 2.82e-40 | 1.81e-40 | 9.98e-41 | 4.01e-41 |
| 5  | 5.87e-39 | 5.60e-39 | 4.96e-39 | 3.86e-39 | 2.54e-39 | 1.50e-39 | 9.45e-40 | 6.13e-40 | 3.80e-40 | 2.44e-40 | 1.30e-40 | 5.19e-41 |
| 6  | 7.46e-39 | 6.73e-39 | 5.89e-39 | 4.38e-39 | 2.85e-39 | 1.69e-39 | 1.09e-39 | 7.32e-40 | 4.64e-40 | 2.94e-40 | 1.57e-40 | 6.50e-41 |
| 7  | 8.63e-39 | 7.60e-39 | 6.27e-39 | 4.62e-39 | 2.98e-39 | 1.82e-39 | 1.21e-39 | 8.35e-40 | 5.32e-40 | 3.41e-40 | 1.80e-40 | 7.49e-41 |
| 8  | 5.01e-39 | 7.78e-39 | 6.27e-39 | 4.47e-39 | 2.86e-39 | 1.83e-39 | 1.29e-39 | 9.30e-40 | 6.07e-40 | 3.92e-40 | 2.07e-40 | 8.55e-41 |
| 9  | 1.21e-40 | 4.87e-39 | 5.21e-39 | 3.64e-39 | 2.42e-39 | 1.67e-39 | 1.28e-39 | 9.78e-40 | 6.61e-40 | 4.30e-40 | 2.27e-40 | 9.47e-41 |
| 10 | 0.00e+00 | 3.25e-40 | 3.11e-39 | 2.59e-39 | 1.85e-39 | 1.42e-39 | 1.14e-39 | 9.26e-40 | 6.48e-40 | 4.24e-40 | 2.29e-40 | 9.77e-41 |
| 11 | 0.00e+00 | 0.00e+00 | 2.19e-40 | 1.16e-39 | 1.23e-39 | 1.04e-39 | 9.06e-40 | 7.80e-40 | 5.69e-40 | 3.89e-40 | 2.13e-40 | 9.40e-41 |
| 12 | 0.00e+00 | 0.00e+00 | 0.00e+00 | 0.00e+00 | 3.47e-40 | 6.17e-40 | 5.91e-40 | 5.37e-40 | 4.24e-40 | 3.06e-40 | 1.77e-40 | 8.40e-41 |
| 13 | 0.00e+00 | 0.00e+00 | 0.00e+00 | 0.00e+00 | 0.00e+00 | 1.93e-41 | 7.47e-41 | 1.17e-40 | 1.37e-40 | 1.24e-40 | 8.77e-41 | 5.15e-41 |

TABLE V. Monte Carlo predicted double differential cross section as a function of  $p_{||}$  (columns) and  $p_T$  (rows) in units of  $\text{cm}^2$  per  $\text{GeV}^2$  per nucleon. This prediction is for GENIE 2.8.4.

|    | 1        | 2        | 3        | 4        | 5        | 6        | 7        | 8        | 9        | 10       | 11       | 12       |
|----|----------|----------|----------|----------|----------|----------|----------|----------|----------|----------|----------|----------|
| 1  | 2.74e-40 | 3.05e-40 | 3.04e-40 | 2.41e-40 | 1.63e-40 | 9.48e-41 | 5.74e-41 | 3.48e-41 | 2.11e-41 | 1.54e-41 | 9.76e-42 | 4.65e-42 |
| 2  | 9.44e-40 | 1.05e-39 | 1.03e-39 | 8.24e-40 | 5.35e-40 | 3.15e-40 | 1.86e-40 | 1.16e-40 | 7.52e-41 | 4.74e-41 | 2.58e-41 | 1.12e-41 |
| 3  | 2.17e-39 | 2.20e-39 | 2.09e-39 | 1.65e-39 | 1.08e-39 | 6.35e-40 | 3.81e-40 | 2.49e-40 | 1.53e-40 | 9.71e-41 | 5.38e-41 | 2.24e-41 |
| 4  | 3.71e-39 | 3.63e-39 | 3.34e-39 | 2.56e-39 | 1.67e-39 | 9.79e-40 | 6.05e-40 | 3.90e-40 | 2.43e-40 | 1.57e-40 | 8.66e-41 | 3.51e-41 |
| 5  | 5.23e-39 | 4.93e-39 | 4.28e-39 | 3.27e-39 | 2.12e-39 | 1.26e-39 | 8.09e-40 | 5.32e-40 | 3.35e-40 | 2.15e-40 | 1.14e-40 | 4.61e-41 |
| 6  | 6.70e-39 | 5.98e-39 | 5.19e-39 | 3.81e-39 | 2.46e-39 | 1.47e-39 | 9.58e-40 | 6.54e-40 | 4.16e-40 | 2.64e-40 | 1.41e-40 | 5.90e-41 |
| 7  | 7.80e-39 | 6.84e-39 | 5.64e-39 | 4.14e-39 | 2.65e-39 | 1.63e-39 | 1.10e-39 | 7.64e-40 | 4.88e-40 | 3.13e-40 | 1.64e-40 | 6.85e-41 |
| 8  | 4.57e-39 | 7.14e-39 | 5.78e-39 | 4.15e-39 | 2.66e-39 | 1.71e-39 | 1.21e-39 | 8.71e-40 | 5.68e-40 | 3.67e-40 | 1.93e-40 | 8.03e-41 |
| 9  | 1.12e-40 | 4.54e-39 | 4.92e-39 | 3.47e-39 | 2.32e-39 | 1.59e-39 | 1.22e-39 | 9.30e-40 | 6.28e-40 | 4.08e-40 | 2.15e-40 | 8.93e-41 |
| 10 | 0.00e+00 | 3.08e-40 | 2.98e-39 | 2.50e-39 | 1.79e-39 | 1.36e-39 | 1.10e-39 | 8.85e-40 | 6.20e-40 | 4.04e-40 | 2.18e-40 | 9.35e-41 |
| 11 | 0.00e+00 | 0.00e+00 | 2.11e-40 | 1.12e-39 | 1.18e-39 | 9.97e-40 | 8.72e-40 | 7.50e-40 | 5.47e-40 | 3.73e-40 | 2.04e-40 | 9.03e-41 |
| 12 | 0.00e+00 | 0.00e+00 | 0.00e+00 | 0.00e+00 | 3.34e-40 | 5.95e-40 | 5.70e-40 | 5.19e-40 | 4.09e-40 | 2.95e-40 | 1.72e-40 | 8.15e-41 |
| 13 | 0.00e+00 | 0.00e+00 | 0.00e+00 | 0.00e+00 | 0.00e+00 | 1.88e-41 | 7.27e-41 | 1.14e-40 | 1.34e-40 | 1.21e-40 | 8.60e-41 | 5.08e-41 |

TABLE VI. Monte Carlo predicted double differential cross section as a function of  $p_{||}$  (columns) and  $p_T$  (rows) in units of  $\text{cm}^2$  per  $\text{GeV}^2$  per nucleon. This prediction is for GENIE 2.8.4 with the addition of a pion tune, and RPA model.

|    | 1        | 2        | 3        | 4        | 5        | 6        | 7        | 8        | 9        | 10       | 11       | 12       |
|----|----------|----------|----------|----------|----------|----------|----------|----------|----------|----------|----------|----------|
| 1  | 2.87e-40 | 3.21e-40 | 3.24e-40 | 2.62e-40 | 1.82e-40 | 1.05e-40 | 6.39e-41 | 3.77e-41 | 2.28e-41 | 1.65e-41 | 1.03e-41 | 4.80e-42 |
| 2  | 1.01e-39 | 1.14e-39 | 1.14e-39 | 9.37e-40 | 6.23e-40 | 3.65e-40 | 2.13e-40 | 1.32e-40 | 8.33e-41 | 5.29e-41 | 2.86e-41 | 1.25e-41 |
| 3  | 2.35e-39 | 2.44e-39 | 2.37e-39 | 1.93e-39 | 1.30e-39 | 7.61e-40 | 4.48e-40 | 2.86e-40 | 1.73e-40 | 1.09e-40 | 6.04e-41 | 2.52e-41 |
| 4  | 3.99e-39 | 3.99e-39 | 3.75e-39 | 2.98e-39 | 1.99e-39 | 1.17e-39 | 7.05e-40 | 4.43e-40 | 2.73e-40 | 1.76e-40 | 9.69e-41 | 3.90e-41 |
| 5  | 5.52e-39 | 5.30e-39 | 4.73e-39 | 3.71e-39 | 2.45e-39 | 1.45e-39 | 9.10e-40 | 5.88e-40 | 3.66e-40 | 2.35e-40 | 1.24e-40 | 5.01e-41 |
| 6  | 6.96e-39 | 6.30e-39 | 5.56e-39 | 4.17e-39 | 2.73e-39 | 1.62e-39 | 1.04e-39 | 6.99e-40 | 4.42e-40 | 2.80e-40 | 1.50e-40 | 6.22e-41 |
| 7  | 7.97e-39 | 7.05e-39 | 5.88e-39 | 4.37e-39 | 2.82e-39 | 1.72e-39 | 1.15e-39 | 7.93e-40 | 5.05e-40 | 3.23e-40 | 1.70e-40 | 7.10e-41 |
| 8  | 4.60e-39 | 7.17e-39 | 5.83e-39 | 4.19e-39 | 2.70e-39 | 1.73e-39 | 1.22e-39 | 8.78e-40 | 5.73e-40 | 3.70e-40 | 1.95e-40 | 8.09e-41 |
| 9  | 1.11e-40 | 4.47e-39 | 4.82e-39 | 3.40e-39 | 2.28e-39 | 1.57e-39 | 1.21e-39 | 9.22e-40 | 6.23e-40 | 4.05e-40 | 2.14e-40 | 8.88e-41 |
| 10 | 0.00e+00 | 3.00e-40 | 2.89e-39 | 2.43e-39 | 1.75e-39 | 1.34e-39 | 1.08e-39 | 8.76e-40 | 6.14e-40 | 4.00e-40 | 2.16e-40 | 9.26e-41 |
| 11 | 0.00e+00 | 0.00e+00 | 2.06e-40 | 1.10e-39 | 1.17e-39 | 9.88e-40 | 8.65e-40 | 7.45e-40 | 5.44e-40 | 3.71e-40 | 2.03e-40 | 8.98e-41 |
| 12 | 0.00e+00 | 0.00e+00 | 0.00e+00 | 0.00e+00 | 3.33e-40 | 5.94e-40 | 5.68e-40 | 5.18e-40 | 4.09e-40 | 2.95e-40 | 1.71e-40 | 8.14e-41 |
| 13 | 0.00e+00 | 0.00e+00 | 0.00e+00 | 0.00e+00 | 0.00e+00 | 1.88e-41 | 7.27e-41 | 1.14e-40 | 1.34e-40 | 1.21e-40 | 8.60e-41 | 5.08e-41 |

TABLE VII. Monte Carlo predicted double differential cross section as a function of  $p_{||}$  (columns) and  $p_T$  (rows) in units of  $\text{cm}^2$  per  $\text{GeV}^2$  per nucleon. This prediction is for GENIE 2.8.4 with the addition of a pion tune, and Valencia 2p2h.

|    | 1        | 2        | 3        | 4        | 5        | 6        | 7        | 8        | 9        | 10       | 11       | 12       |
|----|----------|----------|----------|----------|----------|----------|----------|----------|----------|----------|----------|----------|
| 1  | 3.15e-40 | 3.53e-40 | 3.56e-40 | 2.88e-40 | 1.95e-40 | 1.11e-40 | 6.66e-41 | 4.11e-41 | 2.52e-41 | 1.79e-41 | 1.11e-41 | 5.07e-42 |
| 2  | 1.08e-39 | 1.21e-39 | 1.20e-39 | 9.73e-40 | 6.37e-40 | 3.73e-40 | 2.17e-40 | 1.36e-40 | 8.74e-41 | 5.52e-41 | 2.99e-41 | 1.28e-41 |
| 3  | 2.42e-39 | 2.51e-39 | 2.41e-39 | 1.92e-39 | 1.25e-39 | 7.30e-40 | 4.36e-40 | 2.85e-40 | 1.76e-40 | 1.11e-40 | 6.07e-41 | 2.53e-41 |
| 4  | 4.09e-39 | 4.07e-39 | 3.79e-39 | 2.93e-39 | 1.90e-39 | 1.11e-39 | 6.83e-40 | 4.39e-40 | 2.72e-40 | 1.75e-40 | 9.64e-41 | 3.95e-41 |
| 5  | 5.67e-39 | 5.46e-39 | 4.82e-39 | 3.69e-39 | 2.39e-39 | 1.40e-39 | 8.96e-40 | 5.87e-40 | 3.69e-40 | 2.37e-40 | 1.26e-40 | 5.11e-41 |
| 6  | 7.20e-39 | 6.55e-39 | 5.74e-39 | 4.25e-39 | 2.73e-39 | 1.62e-39 | 1.05e-39 | 7.13e-40 | 4.53e-40 | 2.86e-40 | 1.54e-40 | 6.41e-41 |
| 7  | 8.29e-39 | 7.39e-39 | 6.18e-39 | 4.56e-39 | 2.92e-39 | 1.77e-39 | 1.19e-39 | 8.22e-40 | 5.24e-40 | 3.36e-40 | 1.76e-40 | 7.38e-41 |
| 8  | 4.81e-39 | 7.57e-39 | 6.22e-39 | 4.48e-39 | 2.86e-39 | 1.82e-39 | 1.28e-39 | 9.19e-40 | 5.98e-40 | 3.86e-40 | 2.04e-40 | 8.47e-41 |
| 9  | 1.16e-40 | 4.70e-39 | 5.13e-39 | 3.64e-39 | 2.42e-39 | 1.65e-39 | 1.26e-39 | 9.57e-40 | 6.45e-40 | 4.20e-40 | 2.22e-40 | 9.20e-41 |
| 10 | 0.00e+00 | 3.13e-40 | 3.02e-39 | 2.54e-39 | 1.82e-39 | 1.38e-39 | 1.11e-39 | 8.93e-40 | 6.25e-40 | 4.08e-40 | 2.21e-40 | 9.44e-41 |
| 11 | 0.00e+00 | 0.00e+00 | 2.12e-40 | 1.12e-39 | 1.18e-39 | 9.98e-40 | 8.73e-40 | 7.50e-40 | 5.47e-40 | 3.73e-40 | 2.04e-40 | 9.04e-41 |
| 12 | 0.00e+00 | 0.00e+00 | 0.00e+00 | 0.00e+00 | 3.34e-40 | 5.95e-40 | 5.70e-40 | 5.19e-40 | 4.09e-40 | 2.95e-40 | 1.72e-40 | 8.15e-41 |
| 13 | 0.00e+00 | 0.00e+00 | 0.00e+00 | 0.00e+00 | 0.00e+00 | 1.88e-41 | 7.27e-41 | 1.14e-40 | 1.34e-40 | 1.21e-40 | 8.60e-41 | 5.08e-41 |

TABLE VIII. Monte Carlo predicted double differential cross section as a function of  $p_{||}$  (columns) and  $p_T$  (rows) in units of  $\text{cm}^2$  per  $\text{GeV}^2$  per nucleon. This prediction is for GENIE 2.8.4 with the addition of a pion tune, Valencia 2p2h, and RPA model.

|    | 1        | 2        | 3        | 4        | 5        | 6        | 7        | 8        | 9        | 10       | 11       | 12       |
|----|----------|----------|----------|----------|----------|----------|----------|----------|----------|----------|----------|----------|
| 1  | 3.16e-40 | 3.54e-40 | 3.57e-40 | 2.90e-40 | 1.96e-40 | 1.11e-40 | 6.70e-41 | 4.12e-41 | 2.53e-41 | 1.80e-41 | 1.12e-41 | 5.08e-42 |
| 2  | 1.09e-39 | 1.22e-39 | 1.21e-39 | 9.87e-40 | 6.47e-40 | 3.79e-40 | 2.20e-40 | 1.38e-40 | 8.85e-41 | 5.58e-41 | 3.02e-41 | 1.29e-41 |
| 3  | 2.49e-39 | 2.58e-39 | 2.50e-39 | 2.00e-39 | 1.31e-39 | 7.63e-40 | 4.51e-40 | 2.95e-40 | 1.82e-40 | 1.14e-40 | 6.24e-41 | 2.60e-41 |
| 4  | 4.31e-39 | 4.31e-39 | 4.06e-39 | 3.20e-39 | 2.08e-39 | 1.20e-39 | 7.41e-40 | 4.71e-40 | 2.92e-40 | 1.85e-40 | 1.02e-40 | 4.22e-41 |
| 5  | 6.04e-39 | 5.94e-39 | 5.34e-39 | 4.14e-39 | 2.68e-39 | 1.56e-39 | 9.98e-40 | 6.41e-40 | 4.02e-40 | 2.53e-40 | 1.38e-40 | 5.61e-41 |
| 6  | 7.59e-39 | 7.05e-39 | 6.28e-39 | 4.72e-39 | 3.06e-39 | 1.82e-39 | 1.16e-39 | 7.74e-40 | 4.84e-40 | 3.11e-40 | 1.66e-40 | 6.98e-41 |
| 7  | 8.52e-39 | 7.71e-39 | 6.58e-39 | 4.92e-39 | 3.14e-39 | 1.91e-39 | 1.27e-39 | 8.70e-40 | 5.57e-40 | 3.53e-40 | 1.85e-40 | 7.78e-41 |
| 8  | 4.82e-39 | 7.59e-39 | 6.28e-39 | 4.55e-39 | 2.90e-39 | 1.84e-39 | 1.29e-39 | 9.30e-40 | 6.07e-40 | 3.93e-40 | 2.08e-40 | 8.63e-41 |
| 9  | 1.15e-40 | 4.67e-39 | 5.08e-39 | 3.59e-39 | 2.38e-39 | 1.62e-39 | 1.23e-39 | 9.35e-40 | 6.33e-40 | 4.16e-40 | 2.21e-40 | 9.22e-41 |
| 10 | 0.00e+00 | 3.13e-40 | 3.02e-39 | 2.53e-39 | 1.79e-39 | 1.35e-39 | 1.08e-39 | 8.64e-40 | 6.00e-40 | 3.91e-40 | 2.13e-40 | 9.18e-41 |
| 11 | 0.00e+00 | 0.00e+00 | 2.14e-40 | 1.13e-39 | 1.19e-39 | 1.00e-39 | 8.69e-40 | 7.41e-40 | 5.37e-40 | 3.63e-40 | 1.98e-40 | 8.69e-41 |
| 12 | 0.00e+00 | 0.00e+00 | 0.00e+00 | 0.00e+00 | 3.43e-40 | 6.10e-40 | 5.82e-40 | 5.27e-40 | 4.10e-40 | 2.93e-40 | 1.69e-40 | 7.95e-41 |
| 13 | 0.00e+00 | 0.00e+00 | 0.00e+00 | 0.00e+00 | 0.00e+00 | 1.95e-41 | 7.56e-41 | 1.18e-40 | 1.39e-40 | 1.24e-40 | 8.70e-41 | 5.07e-41 |

TABLE IX. Monte Carlo predicted double differential cross section as a function of  $p_{||}$  (columns) and  $p_T$  (rows) in units of  $\text{cm}^2$  per  $\text{GeV}^2$  per nucleon. This prediction is for MnvGENIE v1 with the nCTEQ15 DIS model used to reweight DIS events.

|    | 1        | 2        | 3        | 4        | 5        | 6        | 7        | 8        | 9        | 10       | 11       | 12       |
|----|----------|----------|----------|----------|----------|----------|----------|----------|----------|----------|----------|----------|
| 1  | 3.16e-40 | 3.54e-40 | 3.57e-40 | 2.90e-40 | 1.96e-40 | 1.11e-40 | 6.70e-41 | 4.12e-41 | 2.53e-41 | 1.80e-41 | 1.12e-41 | 5.08e-42 |
| 2  | 1.09e-39 | 1.22e-39 | 1.21e-39 | 9.87e-40 | 6.47e-40 | 3.79e-40 | 2.20e-40 | 1.38e-40 | 8.85e-41 | 5.58e-41 | 3.02e-41 | 1.29e-41 |
| 3  | 2.49e-39 | 2.58e-39 | 2.50e-39 | 2.00e-39 | 1.31e-39 | 7.63e-40 | 4.51e-40 | 2.95e-40 | 1.82e-40 | 1.14e-40 | 6.24e-41 | 2.60e-41 |
| 4  | 4.31e-39 | 4.32e-39 | 4.06e-39 | 3.20e-39 | 2.08e-39 | 1.20e-39 | 7.41e-40 | 4.71e-40 | 2.92e-40 | 1.85e-40 | 1.02e-40 | 4.22e-41 |
| 5  | 6.04e-39 | 5.95e-39 | 5.34e-39 | 4.14e-39 | 2.68e-39 | 1.56e-39 | 9.98e-40 | 6.41e-40 | 4.02e-40 | 2.53e-40 | 1.38e-40 | 5.61e-41 |
| 6  | 7.58e-39 | 7.05e-39 | 6.28e-39 | 4.72e-39 | 3.06e-39 | 1.82e-39 | 1.16e-39 | 7.74e-40 | 4.85e-40 | 3.11e-40 | 1.66e-40 | 6.98e-41 |
| 7  | 8.51e-39 | 7.70e-39 | 6.58e-39 | 4.92e-39 | 3.14e-39 | 1.91e-39 | 1.27e-39 | 8.71e-40 | 5.58e-40 | 3.53e-40 | 1.85e-40 | 7.78e-41 |
| 8  | 4.80e-39 | 7.57e-39 | 6.27e-39 | 4.54e-39 | 2.90e-39 | 1.84e-39 | 1.29e-39 | 9.30e-40 | 6.08e-40 | 3.94e-40 | 2.08e-40 | 8.64e-41 |
| 9  | 1.14e-40 | 4.63e-39 | 5.04e-39 | 3.56e-39 | 2.36e-39 | 1.60e-39 | 1.21e-39 | 9.26e-40 | 6.30e-40 | 4.15e-40 | 2.21e-40 | 9.25e-41 |
| 10 | 0.00e+00 | 3.10e-40 | 2.98e-39 | 2.50e-39 | 1.76e-39 | 1.33e-39 | 1.05e-39 | 8.45e-40 | 5.88e-40 | 3.85e-40 | 2.11e-40 | 9.12e-41 |
| 11 | 0.00e+00 | 0.00e+00 | 2.10e-40 | 1.11e-39 | 1.17e-39 | 9.77e-40 | 8.47e-40 | 7.22e-40 | 5.23e-40 | 3.54e-40 | 1.93e-40 | 8.50e-41 |
| 12 | 0.00e+00 | 0.00e+00 | 0.00e+00 | 0.00e+00 | 3.37e-40 | 5.99e-40 | 5.70e-40 | 5.15e-40 | 4.00e-40 | 2.85e-40 | 1.64e-40 | 7.73e-41 |
| 13 | 0.00e+00 | 0.00e+00 | 0.00e+00 | 0.00e+00 | 0.00e+00 | 1.94e-41 | 7.50e-41 | 1.18e-40 | 1.38e-40 | 1.23e-40 | 8.54e-41 | 4.94e-41 |

TABLE X. Monte Carlo predicted double differential cross section as a function of  $p_{||}$  (columns) and  $p_T$  (rows) in units of  $\text{cm}^2$  per  $\text{GeV}^2$  per nucleon. This prediction is for MnvGENIE v1 with the nCTEQ $u$  DIS model used to reweight DIS events.

|    | 1        | 2        | 3        | 4        | 5        | 6        | 7        | 8        | 9        | 10       | 11       | 12       |
|----|----------|----------|----------|----------|----------|----------|----------|----------|----------|----------|----------|----------|
| 1  | 3.16e-40 | 3.54e-40 | 3.57e-40 | 2.90e-40 | 1.96e-40 | 1.11e-40 | 6.70e-41 | 4.12e-41 | 2.53e-41 | 1.80e-41 | 1.12e-41 | 5.08e-42 |
| 2  | 1.09e-39 | 1.22e-39 | 1.21e-39 | 9.87e-40 | 6.47e-40 | 3.79e-40 | 2.20e-40 | 1.38e-40 | 8.85e-41 | 5.58e-41 | 3.02e-41 | 1.29e-41 |
| 3  | 2.49e-39 | 2.58e-39 | 2.50e-39 | 2.00e-39 | 1.31e-39 | 7.63e-40 | 4.51e-40 | 2.95e-40 | 1.82e-40 | 1.14e-40 | 6.24e-41 | 2.60e-41 |
| 4  | 4.31e-39 | 4.31e-39 | 4.06e-39 | 3.20e-39 | 2.08e-39 | 1.20e-39 | 7.41e-40 | 4.71e-40 | 2.92e-40 | 1.85e-40 | 1.02e-40 | 4.22e-41 |
| 5  | 6.02e-39 | 5.94e-39 | 5.34e-39 | 4.14e-39 | 2.68e-39 | 1.56e-39 | 9.98e-40 | 6.41e-40 | 4.02e-40 | 2.53e-40 | 1.38e-40 | 5.61e-41 |
| 6  | 7.55e-39 | 7.03e-39 | 6.28e-39 | 4.72e-39 | 3.06e-39 | 1.82e-39 | 1.16e-39 | 7.74e-40 | 4.85e-40 | 3.11e-40 | 1.66e-40 | 6.98e-41 |
| 7  | 8.45e-39 | 7.67e-39 | 6.56e-39 | 4.91e-39 | 3.13e-39 | 1.90e-39 | 1.27e-39 | 8.70e-40 | 5.57e-40 | 3.53e-40 | 1.85e-40 | 7.78e-41 |
| 8  | 4.75e-39 | 7.51e-39 | 6.23e-39 | 4.51e-39 | 2.88e-39 | 1.83e-39 | 1.28e-39 | 9.23e-40 | 6.05e-40 | 3.93e-40 | 2.08e-40 | 8.63e-41 |
| 9  | 1.11e-40 | 4.54e-39 | 4.95e-39 | 3.50e-39 | 2.31e-39 | 1.57e-39 | 1.19e-39 | 9.05e-40 | 6.18e-40 | 4.09e-40 | 2.19e-40 | 9.21e-41 |
| 10 | 0.00e+00 | 3.03e-40 | 2.91e-39 | 2.42e-39 | 1.70e-39 | 1.27e-39 | 1.01e-39 | 8.05e-40 | 5.60e-40 | 3.68e-40 | 2.03e-40 | 8.83e-41 |
| 11 | 0.00e+00 | 0.00e+00 | 2.05e-40 | 1.08e-39 | 1.13e-39 | 9.38e-40 | 8.10e-40 | 6.89e-40 | 4.96e-40 | 3.34e-40 | 1.81e-40 | 7.96e-41 |
| 12 | 0.00e+00 | 0.00e+00 | 0.00e+00 | 0.00e+00 | 3.30e-40 | 5.88e-40 | 5.56e-40 | 4.99e-40 | 3.85e-40 | 2.73e-40 | 1.56e-40 | 7.33e-41 |
| 13 | 0.00e+00 | 0.00e+00 | 0.00e+00 | 0.00e+00 | 0.00e+00 | 1.94e-41 | 7.53e-41 | 1.19e-40 | 1.38e-40 | 1.22e-40 | 8.43e-41 | 4.86e-41 |

TABLE XI. Monte Carlo predicted double differential cross section as a function of  $p_{||}$  (columns) and  $p_T$  (rows) in units of  $\text{cm}^2$  per  $\text{GeV}^2$  per nucleon. This prediction is for MnvGENIE v1 with the AMU DIS model used to reweight DIS events.

|    | 1        | 2        | 3        | 4        | 5        | 6        | 7        | 8        | 9        | 10       | 11       | 12       |
|----|----------|----------|----------|----------|----------|----------|----------|----------|----------|----------|----------|----------|
| 1  | 2.37e-40 | 2.72e-40 | 2.90e-40 | 2.61e-40 | 1.79e-40 | 1.07e-40 | 5.77e-41 | 3.63e-41 | 2.33e-41 | 1.44e-41 | 7.87e-42 | 2.92e-42 |
| 2  | 8.84e-40 | 1.03e-39 | 1.06e-39 | 9.21e-40 | 6.20e-40 | 3.72e-40 | 2.28e-40 | 1.37e-40 | 8.16e-41 | 4.99e-41 | 2.85e-41 | 1.18e-41 |
| 3  | 2.16e-39 | 2.28e-39 | 2.32e-39 | 1.99e-39 | 1.35e-39 | 7.96e-40 | 4.75e-40 | 2.90e-40 | 1.76e-40 | 1.14e-40 | 6.19e-41 | 2.55e-41 |
| 4  | 3.82e-39 | 3.89e-39 | 3.75e-39 | 3.08e-39 | 2.13e-39 | 1.26e-39 | 7.72e-40 | 4.76e-40 | 2.91e-40 | 1.82e-40 | 9.98e-41 | 4.03e-41 |
| 5  | 5.39e-39 | 5.19e-39 | 4.87e-39 | 3.95e-39 | 2.62e-39 | 1.54e-39 | 9.78e-40 | 6.21e-40 | 3.80e-40 | 2.47e-40 | 1.33e-40 | 5.50e-41 |
| 6  | 6.77e-39 | 6.37e-39 | 5.71e-39 | 4.40e-39 | 2.91e-39 | 1.76e-39 | 1.13e-39 | 7.45e-40 | 4.65e-40 | 2.90e-40 | 1.60e-40 | 6.59e-41 |
| 7  | 7.72e-39 | 7.08e-39 | 6.13e-39 | 4.58e-39 | 3.02e-39 | 1.82e-39 | 1.22e-39 | 8.31e-40 | 5.24e-40 | 3.41e-40 | 1.83e-40 | 7.41e-41 |
| 8  | 4.63e-39 | 7.32e-39 | 6.03e-39 | 4.38e-39 | 2.86e-39 | 1.79e-39 | 1.25e-39 | 8.89e-40 | 5.87e-40 | 3.77e-40 | 2.03e-40 | 8.42e-41 |
| 9  | 1.12e-40 | 4.63e-39 | 5.01e-39 | 3.51e-39 | 2.36e-39 | 1.61e-39 | 1.20e-39 | 9.11e-40 | 6.17e-40 | 3.98e-40 | 2.16e-40 | 9.07e-41 |
| 10 | 0.00e+00 | 3.26e-40 | 3.06e-39 | 2.55e-39 | 1.81e-39 | 1.35e-39 | 1.11e-39 | 8.71e-40 | 6.03e-40 | 4.03e-40 | 2.14e-40 | 9.15e-41 |
| 11 | 0.00e+00 | 0.00e+00 | 2.22e-40 | 1.19e-39 | 1.25e-39 | 1.05e-39 | 9.23e-40 | 7.65e-40 | 5.54e-40 | 3.75e-40 | 2.05e-40 | 8.87e-41 |
| 12 | 0.00e+00 | 0.00e+00 | 0.00e+00 | 0.00e+00 | 3.77e-40 | 6.84e-40 | 6.45e-40 | 5.74e-40 | 4.47e-40 | 3.14e-40 | 1.79e-40 | 8.31e-41 |
| 13 | 0.00e+00 | 0.00e+00 | 0.00e+00 | 0.00e+00 | 0.00e+00 | 2.40e-41 | 8.74e-41 | 1.38e-40 | 1.60e-40 | 1.39e-40 | 9.50e-41 | 5.34e-41 |

TABLE XII. Monte Carlo predicted double differential cross section as a function of  $p_{||}$  (columns) and  $p_T$  (rows) in units of  $\text{cm}^2$  per  $\text{GeV}^2$  per nucleon. This prediction is for NuWro 19.02.

|    | 1        | 2        | 3        | 4        | 5        | 6        | 7        | 8        | 9        | 10       | 11       | 12       |
|----|----------|----------|----------|----------|----------|----------|----------|----------|----------|----------|----------|----------|
| 1  | 2.35e-40 | 2.72e-40 | 2.77e-40 | 2.32e-40 | 1.55e-40 | 9.00e-41 | 5.47e-41 | 3.39e-41 | 2.08e-41 | 1.37e-41 | 7.38e-42 | 3.10e-42 |
| 2  | 8.65e-40 | 9.62e-40 | 9.77e-40 | 8.25e-40 | 5.62e-40 | 3.29e-40 | 1.97e-40 | 1.21e-40 | 7.28e-41 | 4.63e-41 | 2.54e-41 | 1.04e-41 |
| 3  | 1.98e-39 | 2.08e-39 | 2.06e-39 | 1.73e-39 | 1.19e-39 | 6.94e-40 | 4.21e-40 | 2.56e-40 | 1.54e-40 | 9.73e-41 | 5.23e-41 | 2.18e-41 |
| 4  | 3.41e-39 | 3.44e-39 | 3.30e-39 | 2.74e-39 | 1.87e-39 | 1.10e-39 | 6.68e-40 | 4.14e-40 | 2.48e-40 | 1.56e-40 | 8.41e-41 | 3.47e-41 |
| 5  | 4.68e-39 | 4.59e-39 | 4.31e-39 | 3.50e-39 | 2.37e-39 | 1.41e-39 | 8.66e-40 | 5.48e-40 | 3.33e-40 | 2.11e-40 | 1.13e-40 | 4.64e-41 |
| 6  | 5.75e-39 | 5.50e-39 | 5.04e-39 | 4.01e-39 | 2.69e-39 | 1.61e-39 | 1.02e-39 | 6.53e-40 | 4.05e-40 | 2.53e-40 | 1.35e-40 | 5.52e-41 |
| 7  | 6.44e-39 | 6.04e-39 | 5.38e-39 | 4.20e-39 | 2.78e-39 | 1.70e-39 | 1.10e-39 | 7.33e-40 | 4.57e-40 | 2.92e-40 | 1.53e-40 | 6.28e-41 |
| 8  | 3.76e-39 | 6.09e-39 | 5.22e-39 | 3.95e-39 | 2.60e-39 | 1.64e-39 | 1.11e-39 | 7.77e-40 | 5.00e-40 | 3.18e-40 | 1.69e-40 | 7.02e-41 |
| 9  | 9.30e-41 | 4.08e-39 | 4.49e-39 | 3.24e-39 | 2.17e-39 | 1.46e-39 | 1.08e-39 | 8.08e-40 | 5.39e-40 | 3.46e-40 | 1.84e-40 | 7.68e-41 |
| 10 | 0.00e+00 | 2.94e-40 | 2.84e-39 | 2.44e-39 | 1.76e-39 | 1.32e-39 | 1.06e-39 | 8.37e-40 | 5.76e-40 | 3.75e-40 | 1.98e-40 | 8.29e-41 |
| 11 | 0.00e+00 | 0.00e+00 | 1.99e-40 | 1.09e-39 | 1.16e-39 | 9.88e-40 | 8.62e-40 | 7.25e-40 | 5.32e-40 | 3.61e-40 | 1.97e-40 | 8.63e-41 |
| 12 | 0.00e+00 | 0.00e+00 | 0.00e+00 | 0.00e+00 | 3.35e-40 | 6.04e-40 | 5.79e-40 | 5.21e-40 | 4.11e-40 | 2.94e-40 | 1.68e-40 | 7.81e-41 |
| 13 | 0.00e+00 | 0.00e+00 | 0.00e+00 | 0.00e+00 | 0.00e+00 | 2.11e-41 | 7.67e-41 | 1.22e-40 | 1.45e-40 | 1.28e-40 | 8.81e-41 | 5.03e-41 |

TABLE XIII. Monte Carlo predicted double differential cross section as a function of  $p_{||}$  (columns) and  $p_T$  (rows) in units of  $\text{cm}^2$  per  $\text{GeV}^2$  per nucleon. This prediction is for GiBUU 2019.

## B. Single Differential Cross Sections

The measured single differential cross section in longitudinal momentum is shown in Table XIV, and in transverse momentum in Table XV. The remainder of the tables show the Monte Carlo single differential cross sections in both longitudinal and transverse momentum.

| Bin | Cross Section | Stat. Unc. | Total Unc. |
|-----|---------------|------------|------------|
| 1   | 3.23e-39      | 3.84e-41   | 3.35e-40   |
| 2   | 4.43e-39      | 4.14e-41   | 3.52e-40   |
| 3   | 4.51e-39      | 4.00e-41   | 3.32e-40   |
| 4   | 3.74e-39      | 3.64e-41   | 2.79e-40   |
| 5   | 2.63e-39      | 3.08e-41   | 2.05e-40   |
| 6   | 1.92e-39      | 2.55e-41   | 1.45e-40   |
| 7   | 1.56e-39      | 2.34e-41   | 1.13e-40   |
| 8   | 1.30e-39      | 1.48e-41   | 9.36e-41   |
| 9   | 9.27e-40      | 8.05e-42   | 6.70e-41   |
| 10  | 6.60e-40      | 7.33e-42   | 4.80e-41   |
| 11  | 3.87e-40      | 2.83e-42   | 2.75e-41   |
| 12  | 1.83e-40      | 1.86e-42   | 1.45e-41   |

TABLE XIV. Measured differential cross section as a function of  $p_{||}$  in units of  $\text{cm}^2$  per  $\text{GeV}$  per nucleon.

| Bin | Cross Section | Stat. Unc | Total Unc. |
|-----|---------------|-----------|------------|
| 1   | 8.14e-40      | 3.47e-41  | 8.79e-41   |
| 2   | 3.20e-39      | 6.62e-41  | 3.03e-40   |
| 3   | 7.58e-39      | 8.55e-41  | 6.53e-40   |
| 4   | 1.26e-38      | 1.43e-40  | 1.07e-39   |
| 5   | 1.73e-38      | 1.79e-40  | 1.43e-39   |
| 6   | 2.04e-38      | 2.09e-40  | 1.57e-39   |
| 7   | 2.24e-38      | 2.47e-40  | 1.73e-39   |
| 8   | 2.15e-38      | 1.61e-40  | 1.56e-39   |
| 9   | 1.58e-38      | 1.47e-40  | 1.14e-39   |
| 10  | 1.13e-38      | 1.25e-40  | 8.32e-40   |
| 11  | 7.54e-39      | 7.57e-41  | 5.65e-40   |
| 12  | 4.72e-39      | 6.31e-41  | 3.81e-40   |
| 13  | 1.46e-39      | 1.63e-41  | 1.33e-40   |

TABLE XV. Measured differential cross section as a function of  $p_T$  in units of  $\text{cm}^2$  per GeV per nucleon.

| Bin | Cross Section |
|-----|---------------|
| 1   | 3.09e-39      |
| 2   | 4.15e-39      |
| 3   | 4.26e-39      |
| 4   | 3.46e-39      |
| 5   | 2.47e-39      |
| 6   | 1.73e-39      |
| 7   | 1.29e-39      |
| 8   | 9.85e-40      |
| 9   | 6.78e-40      |
| 10  | 4.50e-40      |
| 11  | 2.45e-40      |
| 12  | 1.06e-40      |

TABLE XVI. Monte Carlo predicted differential cross section as a function of  $p_{||}$  in units of  $\text{cm}^2$  per GeV per nucleon. This prediction is for MnvGENIE v1.

| Bin | Cross Section |
|-----|---------------|
| 1   | 3.07e-39      |
| 2   | 4.11e-39      |
| 3   | 4.17e-39      |
| 4   | 3.38e-39      |
| 5   | 2.44e-39      |
| 6   | 1.73e-39      |
| 7   | 1.30e-39      |
| 8   | 9.94e-40      |
| 9   | 6.86e-40      |
| 10  | 4.56e-40      |
| 11  | 2.49e-40      |
| 12  | 1.07e-40      |

TABLE XVII. Monte Carlo predicted differential cross section as a function of  $p_{||}$  in units of  $\text{cm}^2$  per GeV per nucleon. This prediction is for GENIE 2.8.4.

| Bin | Cross Section |
|-----|---------------|
| 1   | 2.77e-39      |
| 2   | 3.72e-39      |
| 3   | 3.80e-39      |
| 4   | 3.07e-39      |
| 5   | 2.22e-39      |
| 6   | 1.59e-39      |
| 7   | 1.21e-39      |
| 8   | 9.32e-40      |
| 9   | 6.45e-40      |
| 10  | 4.30e-40      |
| 11  | 2.34e-40      |
| 12  | 1.01e-40      |

TABLE XVIII. Monte Carlo predicted differential cross section as a function of  $p_{||}$  in units of  $\text{cm}^2$  per GeV per nucleon. This prediction is for GENIE 2.8.4 with the addition of a pion tune, and RPA model.

| Bin | Cross Section |
|-----|---------------|
| 1   | 2.87e-39      |
| 2   | 3.84e-39      |
| 3   | 3.92e-39      |
| 4   | 3.20e-39      |
| 5   | 2.32e-39      |
| 6   | 1.65e-39      |
| 7   | 1.23e-39      |
| 8   | 9.48e-40      |
| 9   | 6.54e-40      |
| 10  | 4.35e-40      |
| 11  | 2.37e-40      |
| 12  | 1.03e-40      |

TABLE XIX. Monte Carlo predicted differential cross section as a function of  $p_{||}$  in units of  $\text{cm}^2$  per GeV per nucleon. This prediction is for GENIE 2.8.4 with the addition of a pion tune, and Valencia 2p2h.

| Bin | Cross Section |
|-----|---------------|
| 1   | 2.98e-39      |
| 2   | 4.02e-39      |
| 3   | 4.11e-39      |
| 4   | 3.32e-39      |
| 5   | 2.38e-39      |
| 6   | 1.68e-39      |
| 7   | 1.26e-39      |
| 8   | 9.66e-40      |
| 9   | 6.67e-40      |
| 10  | 4.43e-40      |
| 11  | 2.41e-40      |
| 12  | 1.05e-40      |

TABLE XX. Monte Carlo predicted differential cross section as a function of  $p_{||}$  in units of  $\text{cm}^2$  per GeV per nucleon. This prediction is for GENIE 2.8.4 with the addition of a pion tune, Valencia 2p2h, and RPA model.

| Bin | Cross Section |
|-----|---------------|
| 1   | 3.08e-39      |
| 2   | 4.14e-39      |
| 3   | 4.25e-39      |
| 4   | 3.45e-39      |
| 5   | 2.46e-39      |
| 6   | 1.72e-39      |
| 7   | 1.28e-39      |
| 8   | 9.76e-40      |
| 9   | 6.70e-40      |
| 10  | 4.44e-40      |
| 11  | 2.42e-40      |
| 12  | 1.05e-40      |

TABLE XXI. Monte Carlo predicted differential cross section as a function of  $p_{||}$  in units of  $\text{cm}^2$  per GeV per nucleon. This prediction is for MnvGENIE v1 with the nCTEQ15 DIS model used to reweight DIS events.

| Bin | Cross Section |
|-----|---------------|
| 1   | 2.79e-39      |
| 2   | 3.86e-39      |
| 3   | 4.04e-39      |
| 4   | 3.35e-39      |
| 5   | 2.46e-39      |
| 6   | 1.74e-39      |
| 7   | 1.30e-39      |
| 8   | 9.78e-40      |
| 9   | 6.72e-40      |
| 10  | 4.45e-40      |
| 11  | 2.43e-40      |
| 12  | 1.04e-40      |

TABLE XXIV. Monte Carlo predicted differential cross section as a function of  $p_{||}$  in units of  $\text{cm}^2$  per GeV per nucleon. This prediction is for NuWro 19.02.

| Bin | Cross Section |
|-----|---------------|
| 1   | 3.07e-39      |
| 2   | 4.13e-39      |
| 3   | 4.23e-39      |
| 4   | 3.44e-39      |
| 5   | 2.45e-39      |
| 6   | 1.71e-39      |
| 7   | 1.27e-39      |
| 8   | 9.64e-40      |
| 9   | 6.61e-40      |
| 10  | 4.38e-40      |
| 11  | 2.39e-40      |
| 12  | 1.03e-40      |

TABLE XXII. Monte Carlo predicted differential cross section as a function of  $p_{||}$  in units of  $\text{cm}^2$  per GeV per nucleon. This prediction is for MnvGENIE v1 with the nCTEQ $u$  DIS model used to reweight DIS events.

| Bin | Cross Section |
|-----|---------------|
| 1   | 2.38e-39      |
| 2   | 3.34e-39      |
| 3   | 3.59e-39      |
| 4   | 3.05e-39      |
| 5   | 2.25e-39      |
| 6   | 1.60e-39      |
| 7   | 1.18e-39      |
| 8   | 8.88e-40      |
| 9   | 6.09e-40      |
| 10  | 4.02e-40      |
| 11  | 2.18e-40      |
| 12  | 9.37e-41      |

TABLE XXV. Monte Carlo predicted differential cross section as a function of  $p_{||}$  in units of  $\text{cm}^2$  per GeV per nucleon. This prediction is for GiBUU 2019.

| Bin | Cross Section |
|-----|---------------|
| 1   | 3.06e-39      |
| 2   | 4.10e-39      |
| 3   | 4.20e-39      |
| 4   | 3.40e-39      |
| 5   | 2.41e-39      |
| 6   | 1.68e-39      |
| 7   | 1.24e-39      |
| 8   | 9.42e-40      |
| 9   | 6.45e-40      |
| 10  | 4.27e-40      |
| 11  | 2.33e-40      |
| 12  | 1.01e-40      |

TABLE XXIII. Monte Carlo predicted differential cross section as a function of  $p_{||}$  in units of  $\text{cm}^2$  per GeV per nucleon. This prediction is for MnvGENIE v1 with the AMU DIS model used to reweight DIS events.

| Bin | Cross Section |
|-----|---------------|
| 1   | 1.05e-39      |
| 2   | 3.52e-39      |
| 3   | 7.38e-39      |
| 4   | 1.21e-38      |
| 5   | 1.63e-38      |
| 6   | 1.94e-38      |
| 7   | 2.11e-38      |
| 8   | 1.91e-38      |
| 9   | 1.41e-38      |
| 10  | 9.62e-39      |
| 11  | 6.26e-39      |
| 12  | 3.94e-39      |
| 13  | 1.36e-39      |

TABLE XXVI. Monte Carlo predicted differential cross section as a function of  $p_T$  in units of  $\text{cm}^2$  per GeV per nucleon. This prediction is for MnvGENIE v1.

| Bin | Cross Section |
|-----|---------------|
| 1   | 9.68e-40      |
| 2   | 3.36e-39      |
| 3   | 7.24e-39      |
| 4   | 1.17e-38      |
| 5   | 1.54e-38      |
| 6   | 1.84e-38      |
| 7   | 2.04e-38      |
| 8   | 1.91e-38      |
| 9   | 1.44e-38      |
| 10  | 9.92e-39      |
| 11  | 6.51e-39      |
| 12  | 4.08e-39      |
| 13  | 1.38e-39      |

TABLE XXVII. Monte Carlo predicted differential cross section as a function of  $p_T$  in units of  $\text{cm}^2$  per GeV per nucleon. This prediction is for GENIE 2.8.4.

| Bin | Cross Section |
|-----|---------------|
| 1   | 9.64e-40      |
| 2   | 3.33e-39      |
| 3   | 7.08e-39      |
| 4   | 1.13e-38      |
| 5   | 1.47e-38      |
| 6   | 1.74e-38      |
| 7   | 1.91e-38      |
| 8   | 1.79e-38      |
| 9   | 1.34e-38      |
| 10  | 9.34e-39      |
| 11  | 6.20e-39      |
| 12  | 3.94e-39      |
| 13  | 1.36e-39      |

TABLE XXIX. Monte Carlo predicted differential cross section as a function of  $p_T$  in units of  $\text{cm}^2$  per GeV per nucleon. This prediction is for GENIE 2.8.4 with the addition of a pion tune, and Valencia 2p2h.

| Bin | Cross Section |
|-----|---------------|
| 1   | 9.00e-40      |
| 2   | 2.99e-39      |
| 3   | 6.23e-39      |
| 4   | 1.00e-38      |
| 5   | 1.34e-38      |
| 6   | 1.63e-38      |
| 7   | 1.84e-38      |
| 8   | 1.77e-38      |
| 9   | 1.36e-38      |
| 10  | 9.51e-39      |
| 11  | 6.25e-39      |
| 12  | 3.94e-39      |
| 13  | 1.36e-39      |

TABLE XXVIII. Monte Carlo predicted differential cross section as a function of  $p_T$  in units of  $\text{cm}^2$  per GeV per nucleon. This prediction is for GENIE 2.8.4 with the addition of a pion tune, and RPA model.

| Bin | Cross Section |
|-----|---------------|
| 1   | 1.05e-39      |
| 2   | 3.48e-39      |
| 3   | 7.13e-39      |
| 4   | 1.13e-38      |
| 5   | 1.48e-38      |
| 6   | 1.79e-38      |
| 7   | 1.99e-38      |
| 8   | 1.88e-38      |
| 9   | 1.41e-38      |
| 10  | 9.62e-39      |
| 11  | 6.26e-39      |
| 12  | 3.94e-39      |
| 13  | 1.36e-39      |

TABLE XXX. Monte Carlo predicted differential cross section as a function of  $p_T$  in units of  $\text{cm}^2$  per GeV per nucleon. This prediction is for GENIE 2.8.4 with the addition of a pion tune, Valencia 2p2h, and RPA model.

| Bin | Cross Section |
|-----|---------------|
| 1   | 1.05e-39      |
| 2   | 3.52e-39      |
| 3   | 7.38e-39      |
| 4   | 1.21e-38      |
| 5   | 1.63e-38      |
| 6   | 1.94e-38      |
| 7   | 2.10e-38      |
| 8   | 1.90e-38      |
| 9   | 1.39e-38      |
| 10  | 9.41e-39      |
| 11  | 6.17e-39      |
| 12  | 3.94e-39      |
| 13  | 1.38e-39      |

TABLE XXXI. Monte Carlo predicted differential cross section as a function of  $p_T$  in units of  $\text{cm}^2$  per GeV per nucleon. This prediction is for MnvGENIE v1 with the nCTEQ15 DIS model used to reweight DIS events.

| Bin | Cross Section |
|-----|---------------|
| 1   | 1.05e-39      |
| 2   | 3.52e-39      |
| 3   | 7.38e-39      |
| 4   | 1.21e-38      |
| 5   | 1.63e-38      |
| 6   | 1.94e-38      |
| 7   | 2.10e-38      |
| 8   | 1.89e-38      |
| 9   | 1.36e-38      |
| 10  | 8.92e-39      |
| 11  | 5.73e-39      |
| 12  | 3.70e-39      |
| 13  | 1.35e-39      |

TABLE XXXIII. Monte Carlo predicted differential cross section as a function of  $p_T$  in units of  $\text{cm}^2$  per GeV per nucleon. This prediction is for MnvGENIE v1 with the AMU DIS model used to reweight DIS events.

| Bin | Cross Section |
|-----|---------------|
| 1   | 1.05e-39      |
| 2   | 3.52e-39      |
| 3   | 7.38e-39      |
| 4   | 1.21e-38      |
| 5   | 1.63e-38      |
| 6   | 1.94e-38      |
| 7   | 2.10e-38      |
| 8   | 1.90e-38      |
| 9   | 1.38e-38      |
| 10  | 9.26e-39      |
| 11  | 6.02e-39      |
| 12  | 3.84e-39      |
| 13  | 1.36e-39      |

TABLE XXXII. Monte Carlo predicted differential cross section as a function of  $p_T$  in units of  $\text{cm}^2$  per GeV per nucleon. This prediction is for MnvGENIE v1 with the nCTEQ $u$  DIS model used to reweight DIS events.

| Bin | Cross Section |
|-----|---------------|
| 1   | 8.87e-40      |
| 2   | 3.23e-39      |
| 3   | 7.15e-39      |
| 4   | 1.17e-38      |
| 5   | 1.54e-38      |
| 6   | 1.83e-38      |
| 7   | 2.01e-38      |
| 8   | 1.90e-38      |
| 9   | 1.43e-38      |
| 10  | 1.02e-38      |
| 11  | 7.09e-39      |
| 12  | 4.93e-39      |
| 13  | 2.05e-39      |

TABLE XXXIV. Monte Carlo predicted differential cross section as a function of  $p_T$  in units of  $\text{cm}^2$  per GeV per nucleon. This prediction is for NuWro 19.02.

| Bin | Cross Section |
|-----|---------------|
| 1   | 8.32e-40      |
| 2   | 2.96e-39      |
| 3   | 6.33e-39      |
| 4   | 1.03e-38      |
| 5   | 1.36e-38      |
| 6   | 1.61e-38      |
| 7   | 1.75e-38      |
| 8   | 1.63e-38      |
| 9   | 1.27e-38      |
| 10  | 9.58e-39      |
| 11  | 6.73e-39      |
| 12  | 4.56e-39      |
| 13  | 1.89e-39      |

TABLE XXXV. Monte Carlo predicted differential cross section as a function of  $p_T$  in units of  $\text{cm}^2$  per GeV per nucleon. This prediction is for GiBUU 2019.

### C. $Q^2$ and $W$ Distributions

The average four momentum transfer squared,  $Q^2$ , in each bin for CC events in GENIE 2.8.4 is shown in Fig. 1, defined as  $Q^2 = 2E_\nu(E_\mu - p_\mu \cos(\theta_\mu)) - m_\mu^2$ . Here  $E_\mu$  and  $p_\mu$  are the energy and momentum of the muon respectively,  $E_\nu$  is neutrino energy,  $\theta_\mu$  is the muon angle with respect to the beamline, and  $m_\mu$  is the muon mass. The average invariant mass,  $W$ , per bin for GENIE 2.8.4 is shown in Fig. 2, where  $W = \sqrt{m_N^2 + 2(E_\nu - E_\mu) - Q^2}$  and  $m_N$  is the mass of the nucleon. Standard deviations are shown as the error bands in both figures. The true DIS thresholds, at  $Q^2 = 1 \text{ GeV}^2$  and  $W = 2 \text{ GeV}$ , are marked by dashed lines in the respective figures.

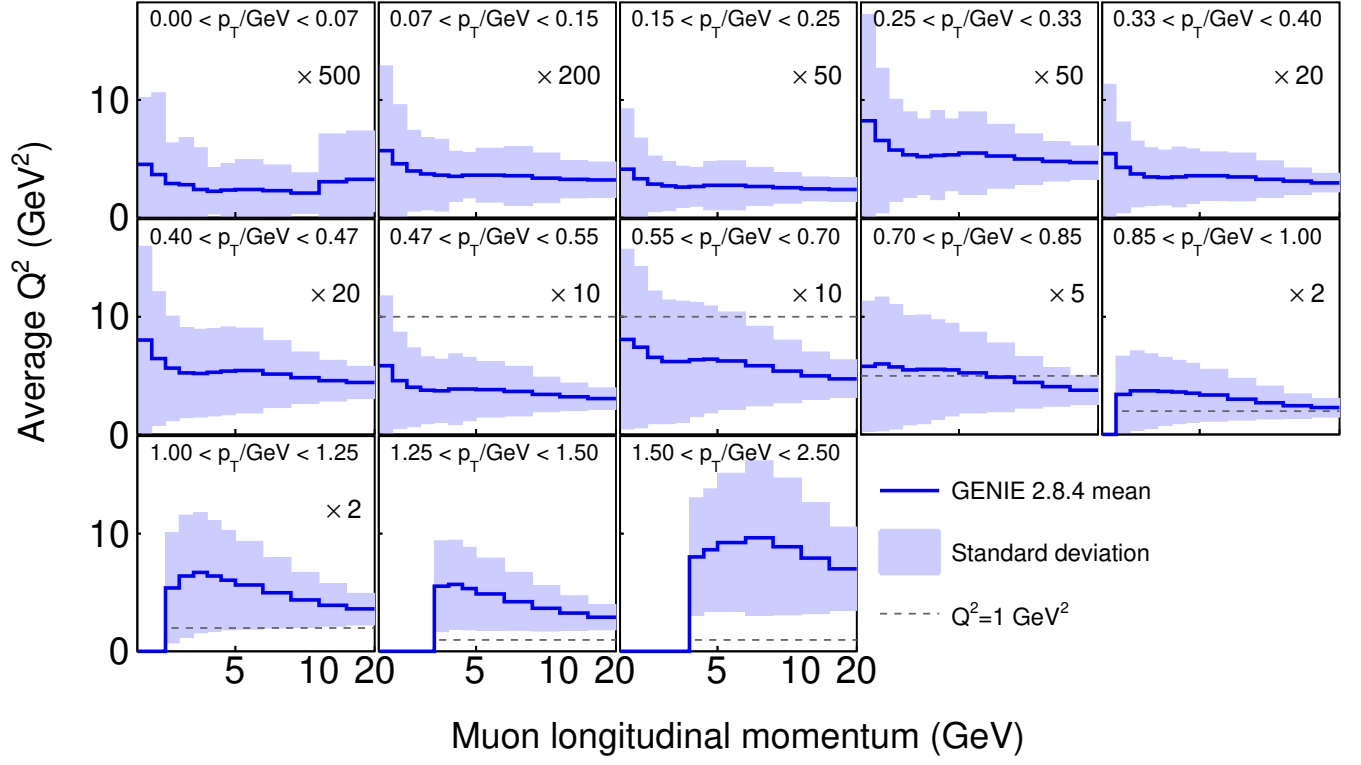

FIG. 1. Average  $Q^2$  of CC interactions for each bin used in this analysis for GENIE 2.8.4, with the standard deviation shown as the error band.

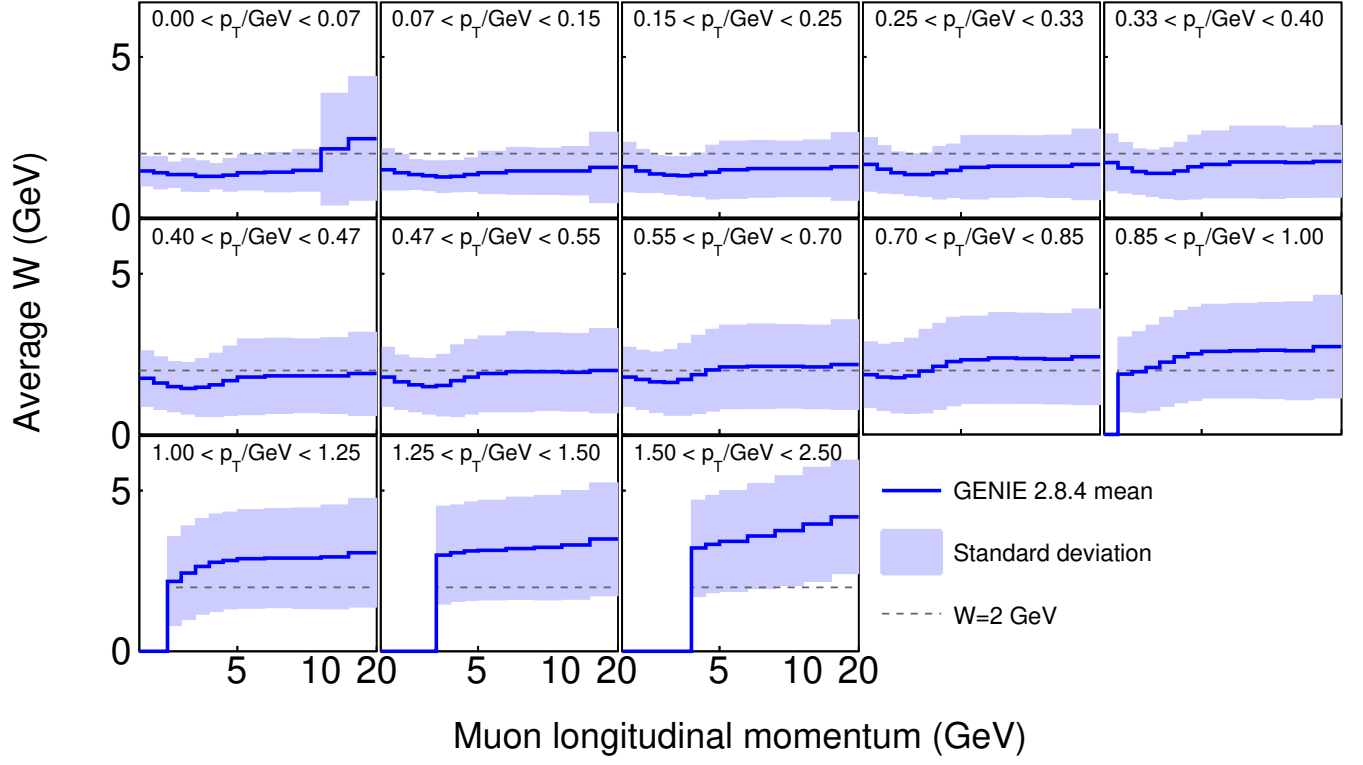

FIG. 2. Average  $W$  of CC interactions for each bin used in this analysis for GENIE 2.8.4, with the standard deviation shown as the error band.
